# Supplementary material for: Versatile tuning of Kerr soliton microcombs in crystalline microresonators
Source: arXiv:2206.13782 ancillary file (2023-03-02)
Supplement: Supplementary file 1 [file Versatile_soliton_tuning_SI_20221205.pdf]

# Supplementary information to "Versatile tuning of Kerr soliton microcombs in crystalline microresonators"

**Shun Fujii[1,2,3,*], Koshiro Wada[3], Ryo Sugano[3], Hajime Kumazaki[3], Soma Kogure[3], Yuichiro K. Kato[2,4], and Takasumi Tanabe[3,*]**

[1]Department of Physics, Faculty of Science and Technology, Keio University, Yokohama, 223-8522, Japan
[2]Quantum Optoelectronics Research Team, RIKEN Center for Advanced Photonics, Saitama 351-0198, Japan
[3]Department of Electronics and Electrical Engineering, Faculty of Science and Technology, Keio University, Yokohama, 223-8522, Japan
[4]Nanoscale Quantum Photonics Laboratory, RIKEN Cluster for Pioneering Research, Saitama 351-0198, Japan
[*]shun.fujii@phys.keio.ac.jp; takasumi@elec.keio.ac.jp

## Supplementary Note 1: Experimental setup for soliton generation

Figure S1(a) shows the experimental setup for soliton generation and the recorded signals. A continuous-wave (CW) fiber laser (NKT Photonics, Koheras ADJUSTIK E15) is modulated by using a fiber-coupled electro-optic modulator (EOM) (Thorlabs, LN65S-FC) and then amplified with an erbium-doped fiber amplifier (PriTel, PMFA-30-IO). The output of a signal generator (SG) (Keysight, E4421B) is sent to both the EOM and a double-balance mixer (DBM) to produce an error signal via the Pound-Drever-Hall (PDH) technique (Fig. S1(b)). An arbitrary waveform generator (AWG) (NF, WF1948) is used to scan the laser frequency and initiate a servo controller by a trigger signal. The low-frequency sideband peak of the PDH signal is used as a lock point (Fig. S1(b)), and the locked detuning can be controlled by changing the modulation frequency applied to the EOM[1,2]. Once the servo initiates the feedback control with proper gain and corner frequency setting, the pump frequency begins to chase the constant detuning frequency to minimize the error signal. A frequency-calibrated Mach-Zehnder interferometer (MZI) provides the time-to-frequency reference signal of the laser frequency, where one period corresponds to 20 MHz. The optical and electrical spectra are observed with an optical spectrum analyzer (OSA) (Yokogawa, AQ6370D) and an electrical spectrum analyzer (ESA) (Rohde & Schwarz, FSW26). The wavelength of the pump laser is monitored with a wavelength meter (WM) (Bristol, 428A). Figure S2(a) and S2(b) show the soliton envelopes when the temperature is increased and the relation between the average soliton power and coupling strength, respectively.

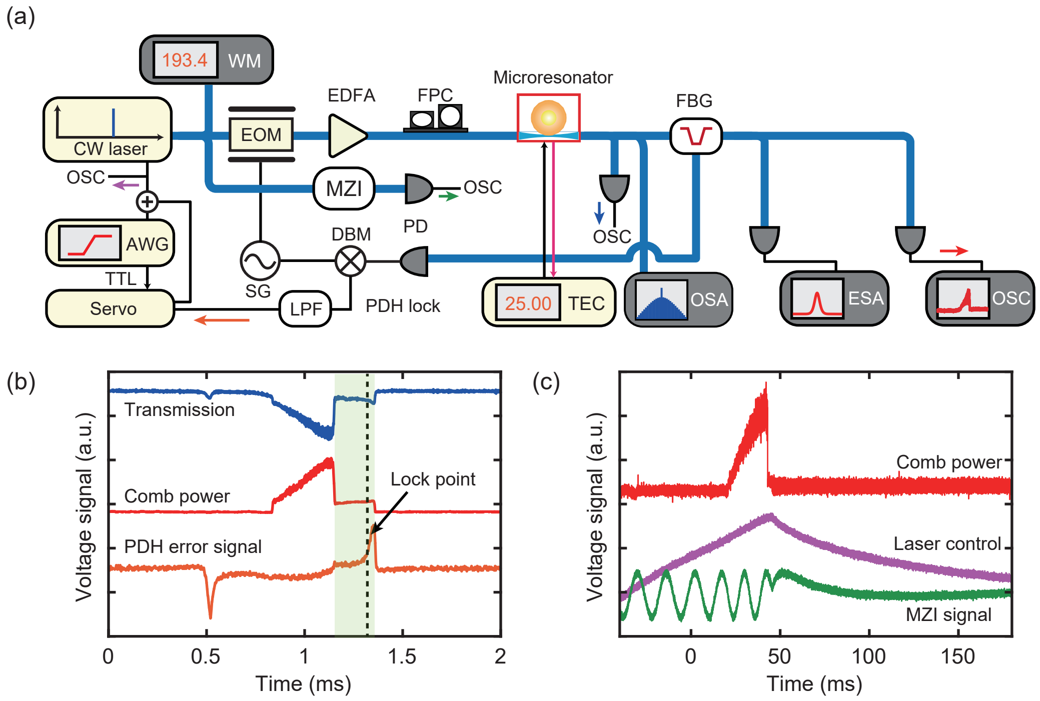


**Supplementary Figure S1.** (a) Experimental setup. OSA: Optical spectrum analyzer; ESA: Electrical spectrum analyzer; OSC: Oscilloscope; FBG: Fiber Bragg grating; TEC: Thermo-electric cooler controller; PD: Photodiode; LPF: Low-pass filter. (b,c) A soliton step is observed in the transmission spectrum (blue) and converted comb power (red). The error signal (orange) is used to stabilize the soliton state via a servo controller. A laser control signal (purple) indicates the change in the laser frequency while activating the servo lock and an MZI signal (green) provides the time-to-frequency reference.

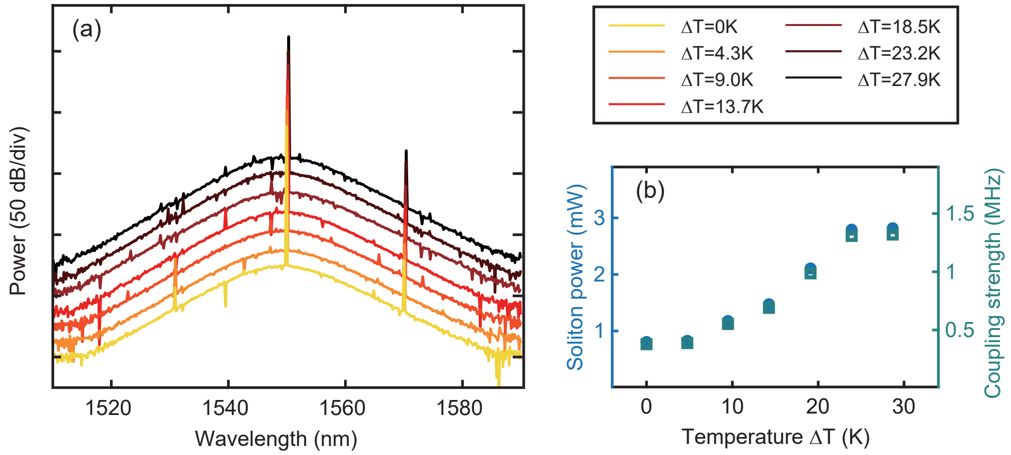


**Supplementary Figure S2.** (a) A sequence of soliton envelopes of a single soliton state as a function of temperature with a detuning of 10.5 MHz. (b) Measured average soliton power (blue dots) and coupling strength $\kappa_{\text{ext}}$ (green symbols) versus temperature change.

## Supplementary Note 2: Effective indices of tapered fiber modes

To obtain the effective index and mode field distribution of a tapered fiber, we begin by solving the wave equation in a cylindrical coordinates system $(r, \phi, z)$[3–6]. The wave equation in the $z$-direction is given as,

$$\left[\frac{\partial^2}{\partial r^2} + \frac{1}{r}\frac{\partial}{\partial r} + \frac{1}{r^2}\frac{\partial^2}{\partial \phi^2} + (k^2 - \beta^2)\right]\left[\begin{array}{c} E_z \\ H_z \end{array}\right] = 0. \tag{S1}$$

Eq. (S1) can be rewritten as the following Bessel differential equation,

$$\frac{\partial^2 \Psi}{\partial r^2} + \frac{1}{r}\frac{\partial \Psi}{\partial r} + \left(k^2 - \beta^2 - \frac{l^2}{r^2}\right)\Psi = 0, \tag{S2}$$

with the variable separation, $[E_z H_z]^T = \Psi(r)\exp(\pm jl\phi)$. Noted that the solution is imposed by the conditional branch on $h^2 = k^2 - \beta^2$; and thus for $h^2 < 0$ (i.e., $r > r_{\text{taper}}$), it is known that the solution of Eq. (S2) is expressed with the $l$-th modified Bessel function. Here, $l$ corresponds to the quantum number describing the order of fiber modes. Assuming that $\Psi(r = \infty) = 0$ and $q^2 = -h^2$ are satisfied, the $z$-components in the cladding mode are given as,

$$E_z = A_{0,\text{clad}} K_l(qr)\exp[j(\omega t + l\phi - \beta z)], \tag{S3}$$
$$H_z = B_{0,\text{clad}} K_l(qr)\exp[j(\omega t + l\phi - \beta z)]. \tag{S4}$$

In the same manner, the solution for $h^2 > 0$ (i.e. $r < r_{\text{taper}}$) is given as,

$$E_z = A_{0,\text{core}} J_l(hr)\exp[j(\omega t + l\phi - \beta z)], \tag{S5}$$
$$H_z = B_{0,\text{core}} J_l(hr)\exp[j(\omega t + l\phi - \beta z)], \tag{S6}$$

where $J_l$ is the Bessel function of the first kind. Other components are calculated directly from $E_z$ and $H_z$ as,

$r < r_{\text{taper}}$ :

$$\left(\begin{array}{c} E_r \\ E_\phi \\ H_r \\ H_\phi \end{array}\right) = \frac{-j\beta}{h^2}\left[\begin{array}{c} A_{0,\text{core}} h J_l'(hr) + \frac{j\omega\mu l}{\beta r} B_{0,\text{core}} J_l(hr) \\ \frac{jl}{r} A_{0,\text{core}} J_l(hr) - \frac{\omega\mu}{\beta} B_{0,\text{core}} h J_l'(hr) \\ B_{0,\text{core}} h J_l'(hr) - \frac{j\omega\varepsilon_1 l}{\beta r} A_{0,\text{core}} J_l(hr) \\ \frac{jl}{r} B_{0,\text{core}} J_l(hr) + \frac{\omega\varepsilon_1}{\beta} A_{0,\text{core}} h J_l'(hr) \end{array}\right] e^{j(\omega t + l\phi - \beta z)}, \tag{S7}$$

$r > r_{\text{taper}}$ :

$$\begin{pmatrix} E_r \\ E_\phi \\ H_r \\ H_\phi \end{pmatrix} = \frac{j\beta}{q^2} \begin{bmatrix} A_{0,\text{clad}} q K_l'(qr) + \frac{j\omega\mu l}{\beta r} B_{0,\text{clad}} K_l(qr) \\ \frac{jl}{r} A_{0,\text{clad}} K_l(qr) - \frac{\omega\mu}{\beta} B_{0,\text{clad}} q K_l'(qr) \\ B_{0,\text{clad}} q K_l'(qr) - \frac{j\omega\varepsilon_1 l}{\beta r} A_{0,\text{clad}} K_l(qr) \\ \frac{jl}{r} B_{0,\text{clad}} K_l(qr) + \frac{\omega\varepsilon_1}{\beta} A_{0,\text{clad}} q K_l'(qr) \end{bmatrix} e^{j(\omega t + l\phi - \beta z)}. \tag{S8}$$

By imposing the continuity condition ($r = r_{\text{taper}}$) for the electric and magnetic fields parallel to the surface of the fiber ($E_\phi$, $E_z$, $H_\phi$, and $H_z$) and applying the boundary condition, the characteristics equation is given as,

$$\left( \frac{J_l'(hr_{\text{taper}})}{hr_{\text{taper}} J_l(hr_{\text{taper}})} + \frac{K_l'(qr_{\text{taper}})}{qr_{\text{taper}} K_l(qr_{\text{taper}})} \right) \left( \frac{n_f^2 J_l'(hr_{\text{taper}})}{hr_{\text{taper}} J_l(hr_{\text{taper}})} + \frac{n_0^2 K_l'(qr_{\text{taper}})}{qr_{\text{taper}} K_l(qr_{\text{taper}})} \right) = l^2 \left[ \left( \frac{1}{qr_{\text{taper}}} \right)^2 + \left( \frac{1}{hr_{\text{taper}}} \right)^2 \right]^2 \left( \frac{\beta}{k_0} \right)^2, \tag{S9}$$

where $n_f$ and $n_0$ are the refractive indices of the core ($n_f = 1.444$) and cladding ($n_0 = 1.000$), respectively. For a given $l$ and a frequency $\omega$, eigenvalues $\beta$ are reduced to a finite number, which gives the six field components for each propagation constant $\beta$. By solving Eq. (S9) for $J_l'(hr_{\text{taper}}))/hr_{\text{taper}} J_l'(hr_{\text{taper}})$, the two class of the solutions referred to as the EH and HE modes:

$$\frac{J_{l+1}'(hr_{\text{taper}}))}{hr_{\text{taper}} J_l'(hr_{\text{taper}})} = \left( \frac{n_f^2 + n_0^2}{2n_f^2} \right) \frac{K_l'(qr_{\text{taper}})}{qr_{\text{taper}} K_l(qr_{\text{taper}})} + \left( \frac{1}{(hr_{\text{taper}})^2} - R' \right), \text{ : EH modes} \tag{S10}$$

$$\frac{J_{l-1}'(hr_{\text{taper}}))}{hr_{\text{taper}} J_l'(hr_{\text{taper}})} = -\left( \frac{n_f^2 + n_0^2}{2n_f^2} \right) \frac{K_l'(qr_{\text{taper}})}{qr_{\text{taper}} K_l(qr_{\text{taper}})} + \left( \frac{1}{(hr_{\text{taper}})^2} - R' \right), \text{ : HE modes} \tag{S11}$$

where

$$R' = \sqrt{ \left( \frac{n_f^2 - n_0^2}{2n_f^2} \right)^2 \left( \frac{K_l'(qr_{\text{taper}})}{qr_{\text{taper}} K_l(qr_{\text{taper}})} \right)^2 + \left( \frac{l\beta}{n_f k_0} \right)^2 \left( \frac{1}{q^2 r_{\text{taper}}^2} + \frac{1}{h^2 r_{\text{taper}}^2} \right)^2 }. \tag{S12}$$

Finally, Eqs. (S10) and (S11) give the effective refractive index (i.e. the propagation constant $\beta$) and the mode profile of the tapered optical fiber as shown in Fig. S3. For the special case of $l = 0$, the HE and EH modes are referred to as TE and TM modes, respectively.

## Supplementary Note 3: Thermally induced variations of coupling length and refractive index

To estimate the change in the effective coupling length via the thermal expansion of a resonator, we perform quantitative calculations of the effective length (i.e., arc length), which should come into contact with a tapered fiber when the resonator radius increases towards the radius direction. Since this model neglects the tensile stress and finite length of the fiber, which are inevitably present in practical experiments, the calculated length would be to some extent over-estimated (close to the upper limit) rather than a rigorous value. In this case, the effective length as a function of temperature change is given as $\Delta l = 2(R + \Delta R) \cdot \arccos(R/(R + \Delta R))$, where $R$ is the resonator radius and $\Delta R = \alpha_{l,o} R \Delta T$ is the increased radius induced by the effect of thermal expansion. If a tapered fiber comes into contact with a resonator at a single point, $\Delta l$ is assumed to be nearly zero. $\alpha_{l,o}$ is the thermal-expansion coefficient for the radial direction of an $MgF_2$ resonator. Figure S4 shows the calculated results for different resonator radii. Although the rate of increase of the effective coupling length depends on the resonator radius, the coupling length can be increased by several to several tens of micrometers with ~30 K temperature change.

Temperature-dependent refractive indices for $MgF_2$ crystal are derived from the following expressions: $\partial n_e/\partial T \approx [0.04183 - 5.63233 \times 10^{-4} T] \times 10^{-5}$ for extraordinary ray and $\partial n_o/\partial T \approx [0.09797 - 5.57293 \times 10^{-4} T] \times 10^{-5}$ for ordinary ray[7]; for fused silica, the temperature-dependent refractive index deviation is given as $\partial n_f/\partial T \approx [1.090 + 3.222 \times 10^{-4} T] \times 10^{-5}$[8]. Figure S5 shows the temperature dependence of the refractive index deviation and refractive index. The refractive indices at 25°C and 1.55 μm are defined as 1.444 for $n_f$, 1.37092 for $n_o$, and 1.38229 for $n_e$.

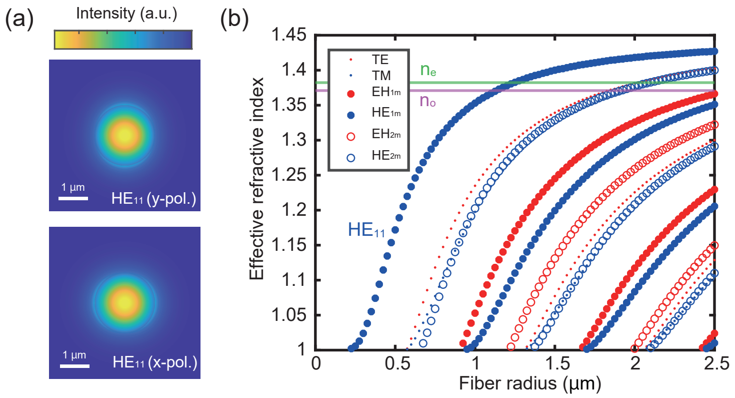


**Supplementary Figure S3.** (a) Mode field distribution of a linearly polarized optical mode ($HE_{11}$) of the tapered optical fiber with a radius of 1 µm. The two images represent the different polarization states. (b) Calculated effective refractive index for the tapered optical fiber with different radii. The purple and green lines indicate the refractive indices of extraordinary and ordinary rays in an $MgF_2$ crystal, respectively. The TE mode, which experiences $n_e$ achieves perfect phase matching with a slightly thicker fiber radius than the TM mode (i.e., $n_o$).

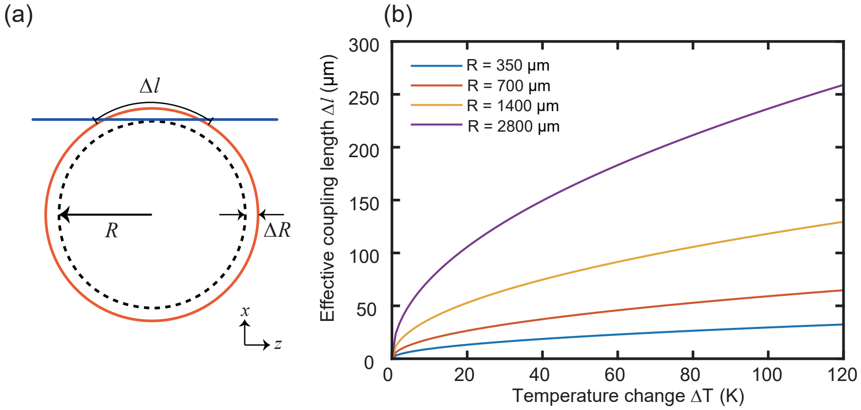


**Supplementary Figure S4.** (a) Schematics of the effect of thermal expansion on the effective coupling length $\Delta l$. The blue line represents a the tangent of the original resonator radius $R$. The thermal expansion effect increases the resonator radius by $\Delta R$ and thus increases $\Delta l$. (b) Effective coupling length $\Delta l$ versus temperature change $\Delta T$. A single point coupling is assumed at $\Delta T = 0$.

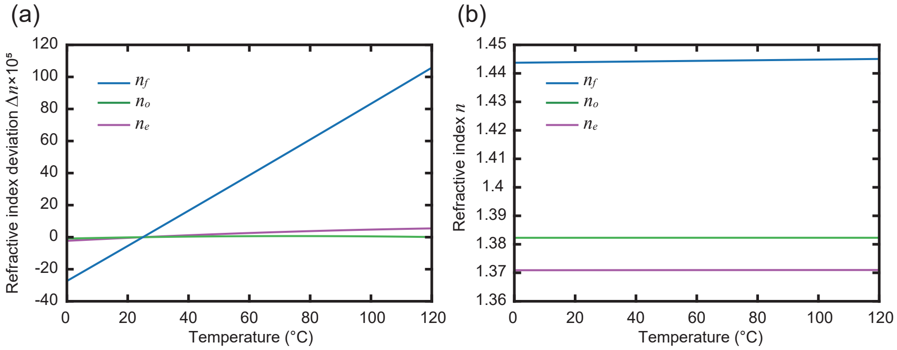


**Supplementary Figure S5.** (a) Temperature dependence of the refractive index deviation of the extraordinary and ordinary rays of $MgF_2$ and fused silica. (b) Temperature dependence of the refractive index of the extraordinary and ordinary rays of $MgF_2$ and fused silica.

## Supplementary Note 4: Coupling strength for fiber-resonator gap

The coupling strength is exponentially reduced when we take account of the physical distance between a tapered fiber and a resonator due to the reduced mode overlap between the two modes. Figure S6 shows the coupling strength as a function of the separation distance for the fundamental (1st) TE and TM modes. The fiber and the resonator are coupled at one point (i.e., $y = 0,\ \varphi = 0$). In practice, it is useful for the fiber to be in full contact with WG resonators with a large diameter for stable light coupling due to the relatively weak leakage of an evanescent field from the resonator. Nevertheless, a separation distance of up to a few micrometers can be employed for microtoroid resonators with a diameter of $\sim$100 µm or other smaller diameter resonators to achieve a critical coupling[9].

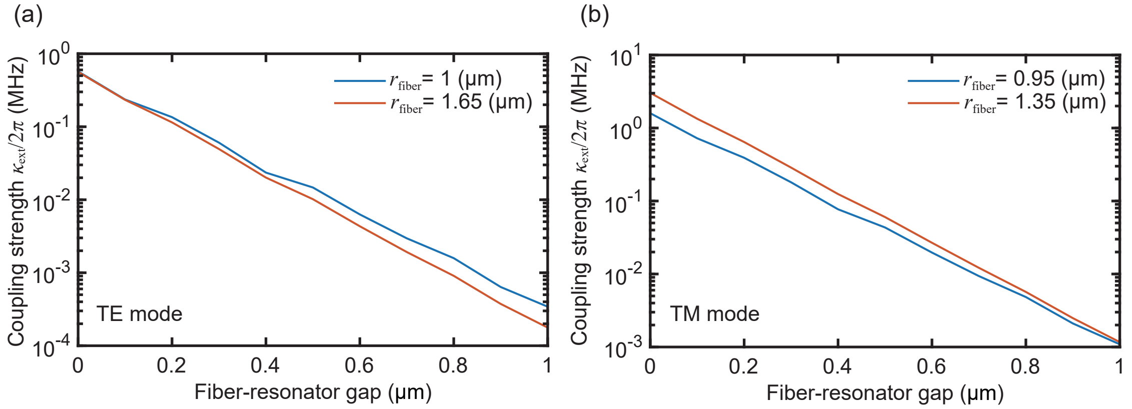


**Supplementary Figure S6.** Coupling strength as a function of the gap between a tapered fiber and a resonator for the 1st TE mode (a) and for the 1st TM mode (b). The fluctuation of the plots is due to the resolution of the FEM simulation.

## Supplementary Note 5: Simulation results for TM polarized mode

The coupling strength for resonator TM modes is shown in Fig. S7. We see that the fiber radius exhibiting the maximum coupling strength is less than with the TE mode owing to the difference of refractive indices. In contrast, the overall trend is similar to that of the TE mode.

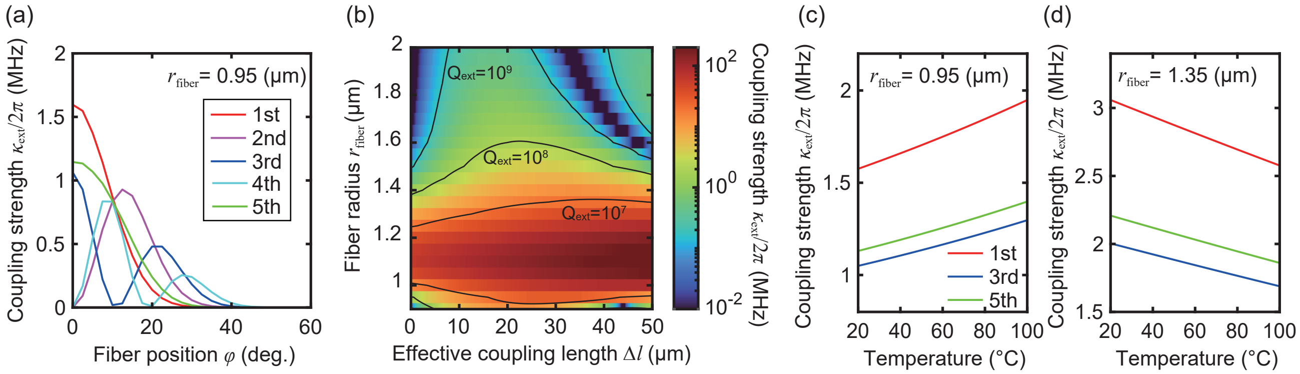


**Supplementary Figure S7.** (a) Coupling strength as a function of fiber position $\varphi$ for TM modes. (b) Contour map of coupling strength showing the dependence on fiber radius and effective coupling length $\Delta l$ for the 1st TM mode. (c, d) Coupling strength as a function of temperature for 1st, 3rd, and 5th TM modes at different fiber radii, (c) for $r_{\rm taper}$ =0.95 µm and (d) for $r_{\rm taper}$ =1.35 µm.

## Supplementary References


**1.** Weng, W. *et al.* Spectral purification of microwave signals with disciplined dissipative kerr solitons. *Physical Review Letters* **122**, 013902 (2019). URL https://link.aps.org/doi/10.1103/PhysRevLett.122.013902.

**2.** Stone, J. R. *et al.* Thermal and nonlinear dissipative-soliton dynamics in Kerr-microresonator frequency combs. *Physical Review Letters* **121**, 063902 (2018). URL https://link.aps.org/doi/10.1103/PhysRevLett.121.063902.

**3.** Yariv, A. *Optical electronics* (Saunders College Publishing, 1991).

**4.** Yariv, A. & Yeh, P. *Photonics: optical electronics in modern communications* (Oxford university press, 2007).

**5.** Humphrey, M. J. *Calculation of coupling between tapered fiber modes and whispering-gallery modes of a spherical microlaser*. Ph.D. thesis, Oklahoma State University (2004).

**6.** Yoshiki, W. *Dynamic control of ultra-high Q silica toroid optical microcavities*. Ph.D. thesis, Keio University (2017).

**7.** Ghosh, G. *Handbook of optical constants of solids: Handbook of thermo-optic coefficients of optical materials with applications* (Academic Press, 1998).

**8.** Gao, H. *et al.* Investigation on the thermo-optic coefficient of silica fiber within a wide temperature range. *Journal of Lightwave Technology* **36**, 5881–5886 (2018). URL https://opg.optica.org/jlt/abstract.cfm?URI=jlt-36-24-5881.

**9.** Spillane, S. M., Kippenberg, T. J., Painter, O. J. & Vahala, K. J. Ideality in a fiber-taper-coupled microresonator system for application to cavity quantum electrodynamics. *Physical Review Letters* **91**, 043902 (2003). URL https://link.aps.org/doi/10.1103/PhysRevLett.91.043902.
